# Supplementary material for: MODIFY: Model-driven Face Stylization without Style Images
Source: arXiv:2303.09831 source file (2023-03-17)
Supplement: Supplementary file 1 [file Appendix.pdf]

# MODIFY: A Model-driven Approach to Privacy-preserving Face Stylization

## Appendix

Anonymous AAAI-2022 Submission

PaperId: 1737

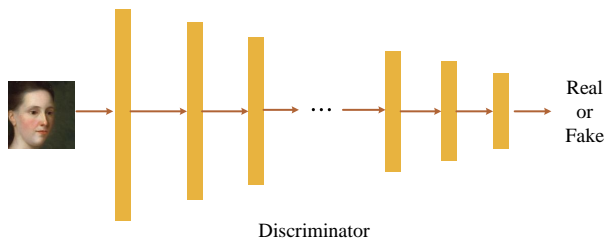

Figure 1: The architecture of the discriminator.

### Discriminator

We build our model upon the official Pytorch implementation of PSP (Elad et al. 2021), from which we inherit most of the training details, including the progressive discriminator proposed by Karras *et al.* (Karras et al. 2017).

### More Visualized Results

We provide more testing results of the comparisons with the state-of-the-art methods in Fig. 2, and results generated from the style-preserving model trained on CUFS and LAMP-HQ in Fig. 4 and Fig. 5, respectively. Fig. 3 shows the noise-

guided results of MODIFY, we are able to generate diverse results from random-selected noise vector.

### References

- Choi, Y.; Uh, Y.; Yoo, J.; and Ha, J.-W. 2020. Stargan v2: Diverse image synthesis for multiple domains. In *Proc. CVPR*.
- Elad, R.; Yuval, A.; Or, P.; Yotam, N.; Yaniv, A.; Stav, S.; and Daniel, C.-O. 2021. Encoding in Style: a StyleGAN Encoder for Image-to-Image Translation. In *Proc. CVPR*.
- Karras, T.; Aila, T.; Laine, S.; and Lehtinen, J. 2017. Progressive growing of gans for improved quality, stability, and variation.
- S, B.; and L., W. 2018. One-Shot Unsupervised Cross Domain Translation. In *Proc. NeurIPS*.
- Copyright © 2022, Association for the Advancement of Artificial Intelligence (www.aaai.org). All rights reserved.
- Wang, X.; and Tang, X. 2008. Face photo-sketch synthesis and recognition. In *IEEE Transactions on Pattern Analysis and Machine Intelligence*.
- Yu, A.; Wu, H.; Huang, H.; Lei, Z.; and He, R. 2021. LAMP-HQ: A Large-Scale Multi-pose High-Quality Database and Benchmark for NIR-VIS Face Recognition. In *International Journal of Computer Vision*.

| (a) Input                  | (b) OST | (c) StarGAN v2 | (d) StarGAN v2 | (e) Unpaired PSP | (f) Unpaired PSP | (g) MODIFY | (h) MODIFY | (i) MODIFY |
|----------------------------|---------|----------------|----------------|------------------|------------------|------------|------------|------------|
| # Samples in $\mathcal{X}$ | 1       | 1              | All            | 1                | All              | 1          | All        | All        |
| Data-driven                | True    | True           | True           | True             | True             | False      | False      | False      |
| Training mode              | Offline | Offline        | Offline        | Offline          | Offline          | Test-time  | Online     | Offline    |

Figure 2: Results of online, offline and test-time training version of MODIFY compared to other three state-of-the-art approaches (*i.e.*, OST (S and L. 2018), StarGAN v2 (Choi et al. 2020), and PSP (Elad et al. 2021)).



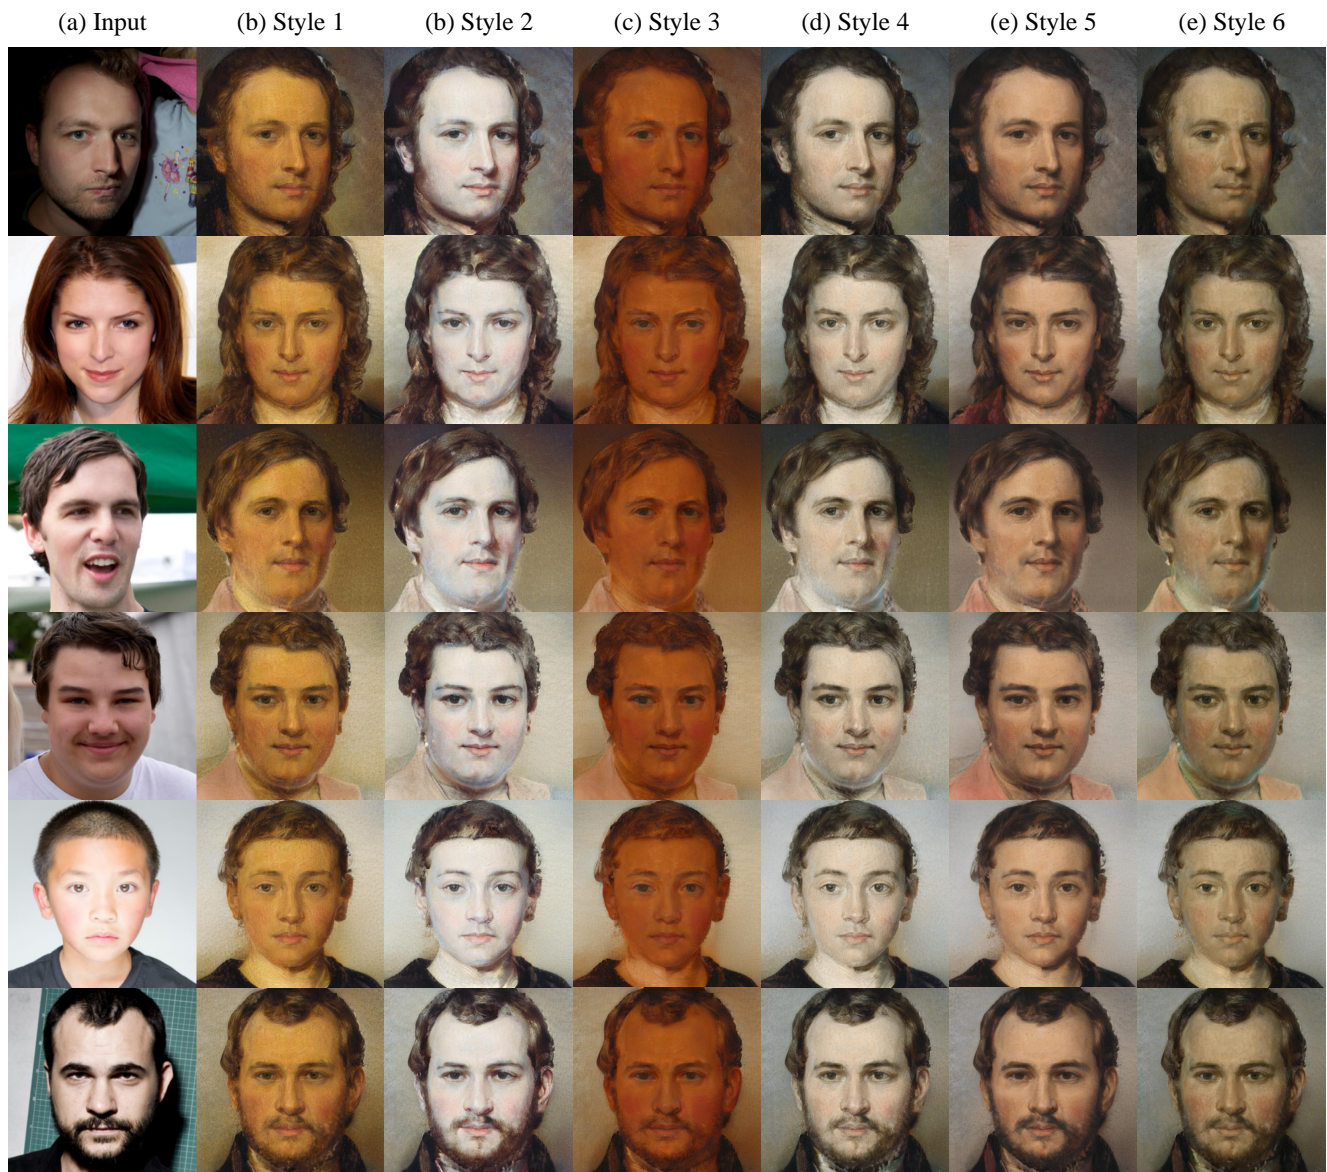

Figure 3: Results generated from different noise vector. Each column generated from the same one.



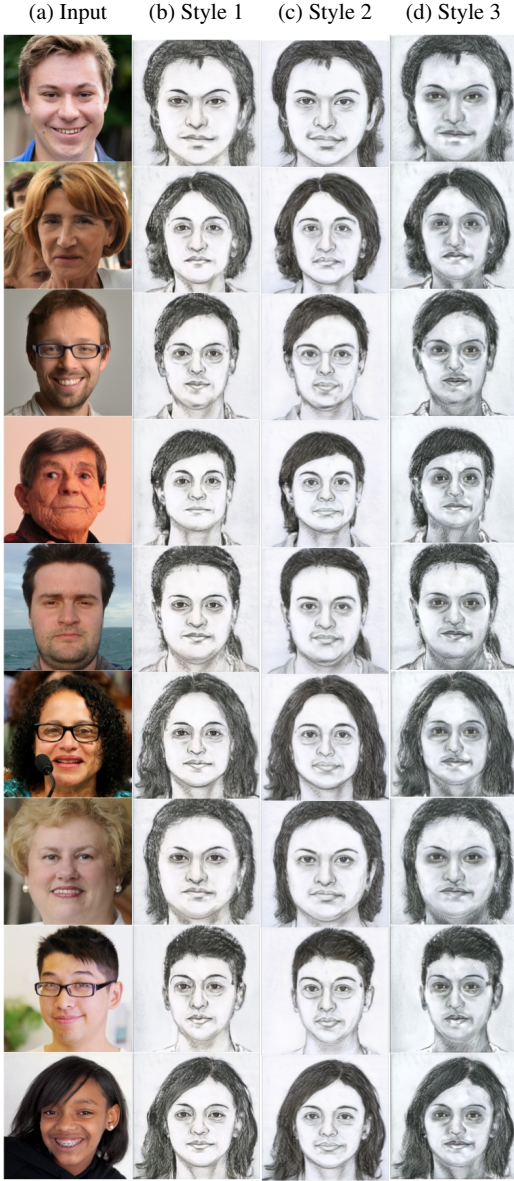

Figure 4: Results generated from the style-preserving model trained on CUFS (Wang and Tang 2008) dataset.

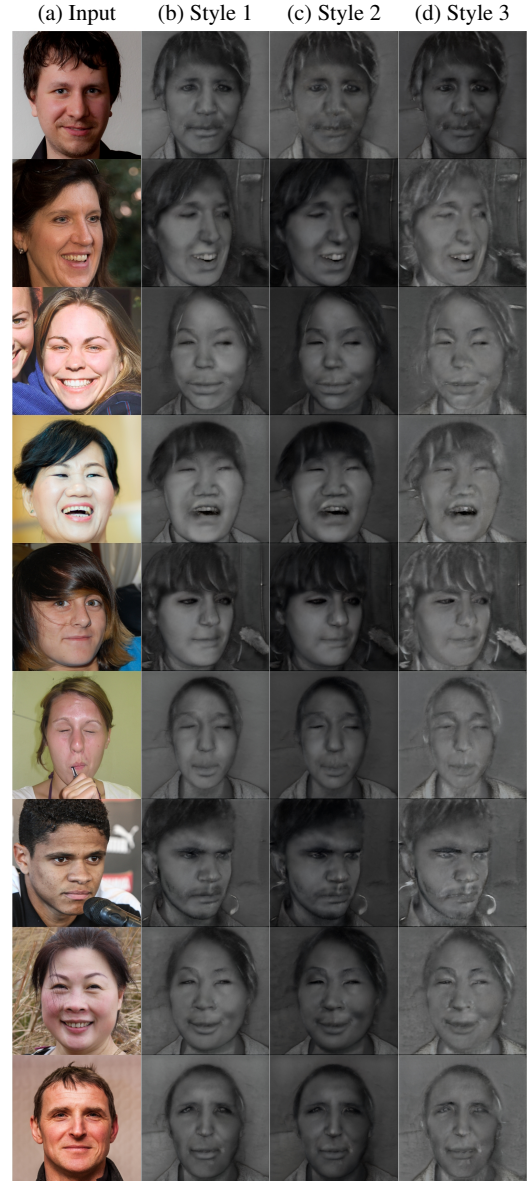

Figure 5: Results generated from the style-preserving model trained on LAMP-HQ (Yu et al. 2021) dataset.
